# Supplementary material for: From Ising to Potts: Physics-inspired Potts machines of coupled oscillators for low-energy sampling and combinatorial optimization
Source: arXiv:2507.18379 source file (2026-01-05)
Supplement: Supplementary file 1 [file SM_OPM.pdf]

# Supplementary Material

# Oscillator Potts machines: An overdamped Langevin model for low-energy sampling of the standard Potts model

Yi Cheng* and Zongli Lin†

*Charles L. Brown Department of Electrical and Computer Engineering,*

*University of Virginia, Charlottesville, Virginia 22904, USA.*

## NOMENCLATURE

| | |
|---|---|
| $\mathbb{R}$ | the set of real numbers |
| $\mathbb{Z}^+$ | the set of positive integers |
| $\mathbb{T}$ | the set of phases in a circle: $[0, 2\pi)$ |
| $\mathbb{R}^N, \mathbb{T}^N$ | the product sets $\mathbb{R} \times \mathbb{R} \times \cdots \times \mathbb{R}$ and $\mathbb{T} \times \mathbb{T} \times \cdots \times \mathbb{T}$ |
| $\imath$ | the unit of imaginary |
| $\Re\{x\}$ | the real part of the complex number $x$ |
| $\Im\{x\}$ | the imaginary part of the complex number $x$ |
| $\mathrm{col}\{x_1, x_2, \ldots, x_N\}$ | $\left[x_1^{\mathrm{T}}\ x_2^{\mathrm{T}}\ \ldots\ x_N^{\mathrm{T}}\right]^{\mathrm{T}}$, with column vectors $\{x_1, x_2, \ldots, x_N\}$ |
| $0_N$ | the $N$-dimensional vector $\mathrm{col}\{0, 0, \ldots, 0\}$ |
| $\nabla U(\theta)$ | the gradient of $U(\theta)$ with respect to $\theta$ |
| $x \in \{a_1, a_2, \ldots, a_m\}^N$ | $x \in \left\{\mathrm{col}\{x_1, x_2, \ldots, x_N\} : x_i \in \{a_1, a_2, \ldots, a_m\}, i = 1, 2, \ldots, N\right\}$ |
| $\|\|x\|\|_\infty$ | the infinity norm of the vector $x$ |
| $\|\|x\|\|_2$ | the 2-norm of the vector $x$ |
| $[-a, +a]_{\theta^\star}^N$ | a hypercube of side $2a$ centered at $\theta^\star \in \mathbb{T}^N$: $\left\{\theta \in \mathbb{T}^N : \|\|\theta - \theta^\star\|\|_\infty \leq a\right\}$ |
| $(-a, +a)_{\theta^\star}^N$ | the interior of $[-a, +a]_{\theta^\star}^N$: $\left\{\theta \in \mathbb{T}^N : \|\|\theta - \theta^\star\|\|_\infty < a\right\}$ |

* zss7gw@virginia.edu

† zl5y@virginia.edu

## I. INTRODUCTION TO DYNAMICS OF OPMS

We begin by detailing the design of the dynamics of OPMs, with the resulting dynamics serving as the subject of our subsequent analysis.

Consider the standard Potts Hamiltonian of $N$ spins,

$$H_{\mathrm{potts}}(s) = -\sum_{i<j} J_{ij}\delta(s_i, s_j),$$

where $s_i \in \{0, 1, \ldots, q-1\}$ is the state of the $i$-th spin, $q \in \mathbb{Z}^+$ is the number of discrete states available to each spin, $J_{ij} \in \mathbb{R}$ is the coupling weights between the $i$-th spin and the $j$-th spin, with $J_{ij} = J_{ji}$ and $J_{ii} = 0$, and

$$\delta(s_i, s_j) = \begin{cases} 1, & \text{if } s_i = s_j, \\ 0, & \text{if } s_i \neq s_j. \end{cases}$$

For the standard Potts model of $N$ spins, the probability of a state $s = \mathrm{col}\{s_1, s_2, \ldots, s_N\}$ under a fixed temperature $T$ follows the Boltzmann distribution,

$$p(s) = Z_{\mathrm{d}}^{-1} \mathrm{e}^{-\beta H_{\mathrm{potts}}(s)},$$

where $\beta = T^{-1}$, $Z_{\mathrm{d}} = \sum_{s\in S} \mathrm{e}^{-\beta H_{\mathrm{potts}}(s)}$, and $S$ is the set of $q^N$ spin configurations. Our goal is to design a Langevin model whose stationary distribution over $q^N$ specified discrete states approximates the Boltzmann distribution or at least is biased to the low-energy spin configurations of the standard Potts Hamiltonian.

For ease in designing the Langevin model, we make a linear transformation for the standard Potts Hamiltonian $H_{\mathrm{potts}}(s)$, that is, $H_{\mathrm{opm}}(s) = (q(q-1)+q)H_{\mathrm{potts}}(s) + \sum_{i<j} J_{ij}q$. It can be verified that $H_{\mathrm{opm}}(s)$ is equal to

$$H_{\mathrm{opm}}(s) = -\sum_{i<j} J_{ij}\tilde{\delta}(s_i, s_j), \tag{1}$$

with

$$\tilde{\delta}(s_i, s_j) = \begin{cases} q(q-1), & \text{if } s_i = s_j, \\ -q, & \text{if } s_i \neq s_j. \end{cases}$$

Instead of considering $H_{\mathrm{potts}}(s)$, we consider its equivalent form $H_{\mathrm{opm}}(s)$ in what follows. Define a potential function $U(\theta)$ as

$$U(\theta) = -\frac{K}{2}\sum_{i<j} J_{ij}\left(2\sum_{m=1}^{q-1}(q-m)\cos(m(\theta_i-\theta_j))\right) - \frac{K_{\mathrm{s}}}{q}\sum_{i=1}^{N}\cos(q\theta_i), \tag{2}$$

where $\theta \in \mathbb{T}^N$, and $K_\mathrm{s}, K > 0$ are tunable parameters. The Langevin model is designed to be

$$\mathrm{d}\theta_t = -\nabla U(\theta_t)\mathrm{d}t + \sqrt{2\beta^{-1}}\mathrm{d}W_t, \tag{3}$$

where the random process $\{\theta_t \in \mathbb{T}^N\}_{t\geq 0}$ is the state and $\mathrm{d}W_t$ is the Wiener process. Expanding (3), we obtain the dynamics of the OPM

$$\begin{aligned}\mathrm{d}[\theta_t]_i = &-\left\{K\sum_{j=1}^{N} J_{ij}\left(\sum_{m=1}^{q-1} m(q-m)\sin(m([\theta_t]_i - [\theta_t]_j))\right) + K_\mathrm{s}\sin(q[\theta_t]_i)\right\}\mathrm{d}t \\ &+\sqrt{2\beta^{-1}}\mathrm{d}W_t,\end{aligned} \tag{4}$$

where $[\theta_t]_i$ is the $i$-th component of $\theta_t$.

The OPM (4) possesses several interesting properties. We will discuss them in detail in the following sections. We first summarize these properties as follows.

- The potential function $U(\theta)$ in discrete states $\theta^\star \in \left\{\frac{2k\pi}{q} : k = 0, 1, \ldots, q-1\right\}^N$ coincides with $H_\mathrm{opm}(s)$ scaled by a factor of $\frac{K}{2}$ in $s \in \{0, 1, \ldots, q-1\}^N$ up to an addictive constant, that is, $U(\theta^\star) = \frac{K}{2}H_\mathrm{opm}(s) + \text{constant}$ (we refer to such discrete states $\theta^\star$ as sampling points).

- In the absence of the Wiener process, the sampling points are structurally stable equilibrium points (EPs) with respect to the coupling weights $J_{ij}$ and the parameters $K$ and $K_\mathrm{s}$.

- In the absence of the Wiener process, the sampling points are only asymptotically stable EPs as $\frac{K_\mathrm{s}}{K} \to \infty$. In addition, the attractive basin of every sampling point $\theta^\star$ converges to a hypercube $\left(-\frac{\pi}{q}, +\frac{\pi}{q}\right)^N_{\theta^\star}$ as $\frac{K_\mathrm{s}}{K} \to \infty$.

- With the Wiener process, if we perform sampling on (4) and then quantize the sampled values to sampling points, then $U(\theta^\star) > U(\phi^\star)$ guarantees that the corresponding $\mathbb{P}_\mathrm{q}(\theta^\star) < \mathbb{P}_\mathrm{q}(\phi^\star)$, where $\mathbb{P}_\mathrm{q}(\theta)$ denotes the probability of $\theta^\star$ occurring after the quantization. That is, when the OPM is used for discrete sampling, the sampling point with lower energy has a higher probability of occurrence.

The first two properties will be discussed in Section II, the third property will be discussed in Section III, and the last property will be discussed in Section IV.

## II. DYNAMIC PROPERTIES OF OPMS

In this section, we focus on dynamic properties of (4) in the absence of the Wiener process,

$$\dot{\theta}_i = -K\sum_{j=1}^{N} J_{ij}\left(\sum_{m=1}^{q-1} m(q-m)\sin(m(\theta_i-\theta_j))\right) - K_{\mathrm{s}}\sin(q\theta_i). \tag{5}$$

Specifically, we comment on the connection between the potential function $U(\theta)$ of (5) and the Potts Hamiltonian $H_{\mathrm{opm}}(s)$, and identify structurally stable EPs of (5).

### A. The potential function $U(\theta)$ and Potts Hamiltonian $H_{\mathrm{opm}}(s)$

An obvious difference between $U(\theta)$ and $H_{\mathrm{opm}}(s)$ is that $U(\theta)$ is a continuous function while $H_{\mathrm{opm}}(s)$ is a discrete function. However, the next theorem shows that the values of $U(\theta)$ at specified discrete points are linearly related to that of $H_{\mathrm{opm}}(s)$

**Theorem 1** *The potential function* (2) *on sampling points* $\theta^\star \in \left\{\frac{2k\pi}{q} : k = 0, 1, \ldots, q-1\right\}^N$ *and the Potts Hamiltonian* (1) *on* $s \in \{0, 1, \ldots, q-1\}^N$ *is related by*

$$U(\theta^\star) = \frac{K}{2}H_{\mathrm{opm}}(s[\theta^\star]) - \frac{K_{\mathrm{s}}N}{q}, \tag{6}$$

*where the mapping* $s[\theta^\star] : \left\{\frac{2k\pi}{q} : k = 0, 1, \ldots, q-1\right\}^N \to \{0, 1, \ldots, q-1\}^N$ *is a component-wise bijection.*

**Remark 1** *The mapping* $s[\theta^\star]$ *is a component-wise bijection, that is, a one-to-one correspondence between the distinct components of* $\theta^\star = \mathrm{col}\{\theta_1^\star, \theta_2^\star, \ldots, \theta_N^\star\}$ *and those of* $s = \mathrm{col}\{s_1, s_2, \ldots, s_N\}$*. Note that the mapping* $s[\theta^\star]$ *is not unique. Without loss of generality, we consider a mapping* $s_i := s_i[\theta^\star] = k$ *if* $\theta_i^\star = \frac{2k\pi}{q}$ *for* $k = 0, 1, \ldots, q-1$*.*

**Proof 1** *The function* $f(x) = 2\sum_{m=1}^{q-1}(q-m)\cos(mx)$ *is a periodic function with the smallest positive period* $T = 2\pi$*. Thus, we only consider* $f(x)$ *for* $x \in \mathbb{T}$*. Clearly, as the sum of an arithmetic sequence,* $f(x) = q(q-1)$ *for* $x = 0$*. We then focus on* $f(x)$ *for* $x \in \left\{\frac{2\pi k}{q} : k = 1, 2, \ldots, q-1\right\}$*. Let* $W_q = \left\{\mathrm{e}^{\imath\frac{2\pi k}{q}} : k = 1, 2, \ldots, q-1\right\}$*. Then, for any* $\omega \in W_q$*,* $\omega^q = 1$ *and* $\sum_{m=1}^{q-1}\omega^m = -1$*. Note that* $f(x)$ *is the real part of*

$$F(x) = 2\sum_{m=1}^{q-1}(q-m)\mathrm{e}^{\imath mx} = 2q\sum_{m=1}^{q-1}\mathrm{e}^{\imath mx} - 2\sum_{m=1}^{q-1}m\mathrm{e}^{\imath mx} := F_1(x) + F_2(x).$$

*For* $x \in \left\{ \frac{2\pi k}{q} : k = 1, 2, \ldots, q-1 \right\}$, *let* $\omega_x = \mathrm{e}^{\imath x}$. *Since* $\omega_x \in W_q$,

$$F_1(x) = 2q \sum_{m=1}^{q-1} \mathrm{e}^{\imath m x} = 2q \sum_{m=1}^{q-1} \omega_x^m = -2q.$$

*Similarly, we have*

$$\begin{aligned} F_2(x) &= -2 \sum_{m=1}^{q-1} m \mathrm{e}^{\imath m x} \\ &= -2 \sum_{m=1}^{q-1} m \omega_x^m \\ &= \frac{-2\omega_x(1 - q\omega_x^{q-1} + (q-1)\omega_x^q)}{(\omega_x - 1)^2} \\ &= \frac{-2(\omega_x - q\omega_x^q + (q-1)\omega_x^{q+1})}{(\omega_x - 1)^2} \\ &= \frac{-2q(\omega_x - 1)}{(\omega_x - 1)^2} \\ &= \frac{-2q}{\omega_x - 1} \\ &= \frac{-2q}{\mathrm{e}^{\imath x} - 1}, \end{aligned}$$

*where, in the third equality, we have used the fact that*

$$\begin{aligned} \sum_{m=1}^{q-1} m\omega_x^m &= \omega_x \frac{\mathrm{d}(\sum_{m=1}^{q-1} \omega_x^m)}{\mathrm{d}\omega_x} \\ &= \frac{\omega_x(1 - q\omega_x^{q-1} + (q-1)\omega_x^q)}{(\omega_x - 1)^2}. \end{aligned}$$

*The real part of* $F_2(x)$ *is given by*

$$\begin{aligned} \Re\{F_2(x)\} &= \Re\left\{ \frac{-2q}{\cos(x) - 1 + \imath \sin(x)} \right\} \\ &= \Re\left\{ \frac{-2q\,(\cos(x) - 1 - \imath \sin(x))}{(\cos(x) - 1)^2 + \sin^2(x)} \right\} \\ &= \Re\left\{ q + \imath \frac{2q \sin(x)}{2 - 2\cos(x)} \right\} \\ &= q. \end{aligned}$$

*Therefore, for* $x \in \left\{ \frac{2\pi k}{q} : k = 1, 2, \ldots, q-1 \right\}$, $f(x) = \Re\{F(x)\} = \Re\{F_1(x)\} + \Re\{F_2(x)\} = -2q + q = -q$. *Then, we obtain*

$$f(x) = \begin{cases} q(q-1), & \text{if } x = 0, \\ -q, & \text{if } x \in \left\{ \frac{2\pi k}{q} : k = 1, 2, \ldots, q-1 \right\}. \end{cases}$$

*Replacing $x$ by $\theta_i^\star - \theta_j^\star$, we yield*

$$f(\theta_i^\star - \theta_j^\star) = \begin{cases} q(q-1), & \text{if } \theta_i^\star - \theta_j^\star = 0, \\ -q, & \text{if } \theta_i^\star - \theta_j^\star \in \left\{ \frac{2\pi k}{q} : k = 1, 2, \ldots, q-1 \right\}. \end{cases}$$

*Since $\theta_i^\star, \theta_j^\star \in \left\{ \frac{2\pi k}{q} : k = 0, 1, \ldots, q-1 \right\}$, the above equation simplifies to*

$$f(\theta_i^\star - \theta_j^\star) = \begin{cases} q(q-1), & \text{if } \theta_i^\star = \theta_j^\star, \\ -q, & \text{if } \theta_i^\star \neq \theta_j^\star. \end{cases}$$

*Note that $s_i[\theta^\star] = k$ if $\theta_i^\star = \frac{2k\pi}{q}$ for $k = 0, 1, \ldots, q-1$. Then, $f(\theta_i^\star - \theta_j^\star) = \tilde{\delta}(s_i[\theta^\star], s_j[\theta^\star])$. In addition, $\cos(q\theta_i^\star) = 1$, and hence $\sum_{i=1}^N \cos(q\theta_i^\star) = N$. Finally, we obtain*

$$\begin{aligned} U(\theta^\star) &= -\frac{K}{2} \sum_{i<j} J_{ij} \left( 2 \sum_{m=1}^{q-1} (q-m) \cos(m(\theta_i - \theta_j)) \right) - \frac{K_\mathrm{s}}{q} \sum_{i=1}^N \cos(q\theta_i) \\ &= -\frac{K}{2} \sum_{i<j} J_{ij} f(\theta_i^\star - \theta_j^\star) - \frac{K_\mathrm{s} N}{q} \\ &= -\frac{K}{2} \sum_{i<j} J_{ij} \tilde{\delta}(s_i[\theta^\star], s_j[\theta^\star]) - \frac{K_\mathrm{s} N}{q} \\ &= \frac{K}{2} H_\mathrm{opm}(s[\theta^\star]) - \frac{K_\mathrm{s} N}{q}. \end{aligned}$$

*This completes the proof.*

**Remark 2** *Based on Theorem 1 and the linear relation between $H_\mathrm{opm}(s)$ and $H_\mathrm{potts}(s)$, we have*

$$U(\theta^\star) = \frac{K\big(q(q-1)+q\big)}{2} H_\mathrm{potts}(s[\theta^\star]) + \frac{K}{2} \sum_{i<j} J_{ij} q - \frac{K_\mathrm{s} N}{q}$$

.

### B. Structurally stable EPs of an OPM

An EP $\theta^\star$ of an OPM is structurally stable if it remains an EP as the coupling weights $J_{ij}$ and the parameters $K$ and $K_\mathrm{s}$ vary. The next theorem identifies the structurally stable EPs of an OPM.

**Theorem 2** *Consider the dynamics* (5).

- *For* $\frac{q}{2} \in \mathbb{Z}^+$, *there are exactly* $2q^N$ *structurally stable EPs. Half of these EPs are sampling points, and the other half belong to* $\left\{\frac{(2k+1)\pi}{q} : k = 0, 1, \ldots, q-1\right\}^N$.

- *For* $\frac{q+1}{2} \in \mathbb{Z}^+$, *there are* $2q^N + q2^N$ *structurally stable EPs, where* $q^N$ *EPs are sampling points,* $q^N$ *EPs belong to* $\left\{\frac{(2k+1)\pi}{q} : k = 0, 1, \ldots, q-1\right\}^N$, *and* $q2^N$ *EPs belong to* $\left\{\frac{k\pi}{q}, \frac{k\pi}{q} + \pi\right\}^N$ *for* $k = 0, 1, \ldots, q-1$.

**Proof 2** *Let* $\theta^\star$ *be a structurally stable EP. Since* $\theta^\star$ *exists for any values of* $J_{ij}$, $K$ *and* $K_{\mathrm{s}}$, *the following equations hold*

$$\sum_{m=1}^{q-1} m(q-m)\sin(m(\theta_i^\star - \theta_j^\star)) = 0, \tag{7}$$

$$\sin(q\theta_i^\star) = 0. \tag{8}$$

*First, it can be verified that*

$$\theta_i^\star \in \left\{\frac{k\pi}{q} : k = 0, 1, \ldots, 2q-1\right\} \tag{9}$$

*is the solution to* (8). *Note that for any* $\theta_i^\star, \theta_j^\star \in \left\{\frac{k\pi}{q} : k = 0, 1, \ldots, 2q-1\right\}$, $\theta_i^\star - \theta_j^\star \in \left\{\frac{k\pi}{q} : k = 0, 1, \ldots, 2q-1\right\}$. *We next show that, for* $\frac{q}{2} \in \mathbb{Z}^+$, *all the solutions to* (7) *are given by* $\theta_i^\star - \theta_j^\star \in \left\{\frac{2k\pi}{q} : k = 0, 1, \ldots, q-1\right\}$, *and, for* $\frac{q+1}{2} \in \mathbb{Z}^+$, *all the solutions to* (7) *are given by* $\theta_i^\star - \theta_j^\star \in \left\{\frac{2k\pi}{q} : k = 0, 1, \ldots, q-1\right\} \bigcup \{\pi\}$.

*Consider the function* $f(x) = \sum_{m=1}^{q-1} m(q-m)\sin(mx)$. *Note that* $f(x)$ *is the imaginary part of*

$$\begin{aligned} F(x) &= \sum_{m=1}^{q-1} m(q-m)\mathrm{e}^{\imath mx} \\ &= q\sum_{m=1}^{q-1} m\mathrm{e}^{\imath mx} - \sum_{m=1}^{q-1} m^2\mathrm{e}^{\imath mx} \\ &:= F_1(x) + F_2(x). \end{aligned}$$

*For* $x = 0$, $F(x) = \sum_{m=1}^{q-1} m(q-m) \in \mathbb{R}$, *and thus* $f(x) = \Im\{F(x)\} = 0$. *For* $x \in \left\{\frac{2k\pi}{q} : k = 1, 2, \ldots, q-1\right\}$, *let* $\omega_x = \mathrm{e}^{\imath x}$. *Then*

$$F_1(x) = q\sum_{m=1}^{q-1} m\mathrm{e}^{\imath mx}$$

$$= q\sum_{m=1}^{q-1} m\omega_x^m$$
$$= \frac{q^2}{\omega_x - 1},$$

*where we have used the fact that*

$$\sum_{m=1}^{q-1} m\omega_x^m = \omega_x \frac{\mathrm{d}(\sum_{m=1}^{q-1}\omega_x^m)}{\mathrm{d}\omega_x}$$
$$= \frac{\omega_x(1 - q\omega_x^{q-1} + (q-1)\omega_x^q)}{(\omega_x - 1)^2}.$$

*Similarly, we have*

$$F_2(x) = -\sum_{m=1}^{q-1} m^2 \mathrm{e}^{\imath m x}$$
$$= -\sum_{m=1}^{q-1} m^2 \omega_x^m$$
$$= -\frac{\omega_x(\omega_x + 1) - \omega_x^q(q^2 - (2q^2 - 2q - 1)\omega_x + (q-1)^2\omega_x^2)}{(1 - \omega_x)^3}$$
$$= \frac{(2q - q^2)\omega_x + q^2}{(\omega_x - 1)^2},$$

*where, in the third equality, we have used the fact that*

$$\sum_{m=1}^{q-1} m^2\omega_x^m = \omega_x \frac{\mathrm{d}\left(\sum_{m=1}^{q-1} m\omega_x^m\right)}{\mathrm{d}\omega_x}$$
$$= \frac{\omega_x(\omega_x + 1) - \omega_x^q(q^2 - (2q^2 - 2q - 1)\omega_x + (q-1)^2\omega_x^2)}{(1 - \omega_x)^3}.$$

*Thus,*

$$F(x) = F_1(x) + F_2(x)$$
$$= \frac{q^2}{\omega_x - 1} + \frac{(2q - q^2)\omega_x + q^2}{(\omega_x - 1)^2}$$
$$= \frac{2q}{\omega_x + \omega_x^{-1} - 2}$$
$$= \frac{q}{\cos(x) - 1}.$$

*Then, we obtain* $f(x) = \Im\{F(x)\} = 0$*. Similarly, for* $x \in \left\{\frac{(2k+1)\pi}{q} : k = 0, 1, \ldots, q-1\right\}$*, let* $\omega_x = \mathrm{e}^{\imath x}$*. Note that in this case,* $\omega_x^q = -1$*. We obtain*

$$F_1(x) = \frac{q(2-q)\omega_x + q^2}{(\omega_x - 1)^2},$$

$$F_2(x) = -\frac{(q^2+2-2q)\omega_x^2 - (2q^2-2q-2)\omega_x + q^2}{(1-\omega_x)^3}.$$

*Then,*

$$\begin{aligned} F(x) &= F_1(x) + F_2(x) \\ &= \frac{-2\omega_x(1+\omega_x)}{(1-\omega_x)^3} \\ &= \imath \frac{\cos\left(\frac{x}{2}\right)}{2\sin^3\left(\frac{x}{2}\right)}, \end{aligned}$$

*where we have used the facts that* $1 - \omega_x = 1 - \mathrm{e}^{\imath x} = -2\imath \mathrm{e}^{\imath \frac{x}{2}} \sin(\frac{x}{2})$ *and* $\omega_x(1+\omega_x) = 2\mathrm{e}^{\imath\frac{3x}{2}}\cos(\frac{x}{2})$*. Thus,*

$$f(x) = \Im\{F(x)\} = \frac{\cos\left(\frac{x}{2}\right)}{2\sin^3\left(\frac{x}{2}\right)},$$

*which is equal to zero if* $x = \pi$*. As a result, we conclude that for* $x \in \left\{\frac{k\pi}{q} : k = 0, 1, \ldots, 2q-1\right\}$,

$$f(x) = 0 \text{ if } x \in \left\{\frac{2k\pi}{q} : k = 0, 1, \ldots, q-1\right\} \bigcup \{\pi\}.$$

*Note that, for* $\frac{q}{2} \in \mathbb{Z}^+$,

$$\left\{\frac{2k\pi}{q} : k = 0, 1, \ldots, q-1\right\} \bigcup \{\pi\} = \left\{\frac{2k\pi}{q} : k = 0, 1, \ldots, q-1\right\},$$

*and hence*

$$f(x) = 0, \quad x \in \left\{\frac{2k\pi}{q} : k = 0, 1, \ldots, q-1\right\}.$$

*Replace* $x$ *by* $\theta_i^\star - \theta_j^\star$*. We have that, if* $\frac{q}{2} \in \mathbb{Z}^+$*, then the solution to* (7) *is given by*

$$\theta_i^\star - \theta_j^\star \in \left\{\frac{2k\pi}{q} : k = 0, 1, \ldots, q-1\right\}, \tag{10}$$

*and if* $\frac{q+1}{2} \in \mathbb{Z}^+$*, then the solution to* (7) *is given by*

$$\theta_i^\star - \theta_j^\star \in \left\{\frac{2k\pi}{q} : k = 0, 1, \ldots, q-1\right\} \bigcup \{\pi\}. \tag{11}$$

*For* $\frac{q}{2} \in \mathbb{Z}^+$*, since* $\theta_i^\star$ *and* $\theta_j^\star$ *satisfy both* (9) *and* (10)*, it can be verified that either* $\theta^\star \in \left\{\frac{2k\pi}{q} : k = 0, 1 \ldots, q-1\right\}^N$ *or* $\theta^\star \in \left\{\frac{(2k+1)\pi}{q} : k = 0, 1, \ldots, q-1\right\}^N$*. Clearly, there are* $2q^N$ *such points. For* $\frac{q+1}{2} \in \mathbb{Z}^+$*, since* $\theta_i^\star$ *and* $\theta_j^\star$ *satisfy both* (9) *and* (11)*, it can be verified that either* $\theta^\star \in \left\{\frac{2k\pi}{q} : k = 0, 1, \ldots, q-1\right\}^N$, $\theta^\star \in \left\{\frac{(2k+1)\pi}{q} : k = 0, 1, \ldots, q-1\right\}^N$*, or* $\theta^\star \in \left\{\frac{k\pi}{q}, \frac{k\pi}{q} + \pi\right\}^N$ *for* $k = 0, 1, \ldots, q-1$*. Clearly, there are* $2q^N + q2^N$ *such points. This completes the proof.*

## III. STABILITY ANALYSIS OF EPS

In this section, we focus on the stability of EPs of an OPM (5). Theorem 2 shows that many other EPs also exhibit structural stability in addition to sampling points. We note that there are also structurally unstable EPs in (5), although they are difficult to locate. We refer to those structurally stable EPs that are not the sampling points as Type I non-sampling points. On the other hand, we refer to structurally unstable EPs as Type II non-sampling points. In practice, those non-sampling points are unwanted. The next theorem shows that all non-sampling points either are unstable or disappear for large enough $\frac{K_{\rm s}}{K}$. In contrast, all sampling points are asymptotically stable for large enough $\frac{K_{\rm s}}{K}$.

**Theorem 3** *Consider the dynamics* (5)*. All the sampling points, the Type I non-sampling points, and the Type II non-sampling points are asymptotically stable, unstable, and either unstable or nonexistent, respectively, for large enough* $\frac{K_{\rm s}}{K}$*.*

**Proof 3** *Given an EP* $\theta^\star$*, the Jacobian matrix of the dynamics* (5) *at* $\theta^\star$ *is given by*

$$A(\theta^\star) = KD(\theta^\star) - qK_{\rm s}\Delta(\theta^\star), \tag{12}$$

*where* $D(\theta^\star)$ *is a symmetric matrix, with diagonal elements*

$$D_{ii}(\theta^\star) = -\sum_{j=1}^{N} J_{ij}\left(\sum_{m=1}^{q-1} m^2(q-m)\cos(m(\theta_i^\star - \theta_j^\star))\right)$$

*and off-diagonal elements*

$$D_{ij}(\theta^\star) = J_{ij}\sum_{m=1}^{q-1} m^2(q-m)\cos(m(\theta_i^\star - \theta_j^\star)),$$

*and* $\Delta(\theta^\star)$ *is a diagonal matrix with* $\Delta_{ii}(\theta^\star) = \cos(q\theta_i^\star)$*. If* $\theta^\star$ *is a sampling point, then* (12) *can be written as* $A(\theta^\star) = KD(\theta^\star) - qK_{\rm s}I_N$*, which is negative definite if and only if*

$$\frac{K_{\rm s}}{K} > \frac{\lambda_N D(\theta^\star)}{q}.$$

*Choosing* $\frac{K_{\rm s}}{K} > \max_{\theta^\star\in\Theta_1}\left\{\frac{\lambda_N D(\theta^\star)}{q}\right\}$*, where* $\Theta_1$ *is the set of* $q^N$ *sampling points, makes all sampling points asymptotically stable. If* $\theta^\star$ *is a Type I non-sampling point, the corresponding Jacobian matrix is* $A(\theta^\star) = KD(\theta^\star) - qK_{\rm s}\Delta(\theta^\star)$*, with at least one diagonal entry of* $\Delta(\theta^\star)$*, say* $\Delta_{11}(\theta^\star)$*, equal to* $-1$*. Thus,* $A_{11}(\theta^\star) = KD_{11}(\theta^\star) + qK_{\rm s}$*, which is positive if* $\frac{K_{\rm s}}{K} > \frac{-D_{11}(\theta^\star)}{q}$*.*

*Choosing* $\frac{K_\mathrm{s}}{K} > \max_{\theta^\star\in\Theta_2}\left\{\frac{-D_{11}(\theta^\star)}{q}\right\}$*, where* $\Theta_2$ *is the set of all Type I non-sampling points, makes all Type I non-sampling points unstable. If* $\theta^\star$ *is a Type II non-sampling point, we consider two cases. In the first case,* $\theta^\star \in \left\{\frac{k\pi}{q} : k = 0, 1, \ldots, 2q-1\right\}^N$*, and there are at least two components of* $\theta^\star$ *in* $\left\{\frac{2k\pi}{q} : 0, 1, \ldots, q-1\right\}$ *and* $\left\{\frac{(2k+1)\pi}{q} : k = 0, 1, \ldots, q-1\right\}$ *each. Since there is at least one phase, say* $\theta_1^\star$*, in* $\left\{\frac{(2k+1)\pi}{q} : k = 0, 1, \ldots, q-1\right\}$*, the instability of the point for large enough* $\frac{K_\mathrm{s}}{K}$ *follows the same argument of that of Type I non-sampling points. In the second case,* $\theta_i^\star \notin \left\{\frac{k\pi}{q} : k = 0, 1, \ldots, 2q-1\right\}$ *for at least one* $i$*,* $i = 1, 2, \ldots, N$*. For such phases, they satisfy*

$$-K\sum_{j=1}^{N} J_{ij}\left(\sum_{m=1}^{q-1} m(q-m)\sin(m(\theta_i^\star - \theta_j^\star))\right) = K_\mathrm{s}\sin(q\theta_i^\star) \neq 0,$$

*that is,*

$$\begin{aligned}\sin(q\theta_i^\star) &= -\frac{K}{K_\mathrm{s}}\sum_{j=1}^{N} J_{ij}\left(\sum_{m=1}^{q-1} m(q-m)\sin(m(\theta_i^\star - \theta_j^\star))\right)\\ &:= -\frac{K}{K_\mathrm{s}}\sum_{j=1}^{N} J_{ij} f(\theta_i^\star - \theta_j^\star) \neq 0.\end{aligned}$$

*Note that* $f(\theta_i - \theta_j)$ *is uniformly bounded with respect to* $\theta_i - \theta_j$*. Let* $\rho_{ij} := \sup_{\theta_i,\theta_j} |J_{ij} f(\theta_i - \theta_j)|$*, and* $\rho_i = \sum_{j=1}^N \rho_{ij} < \infty$*. Note that, by the triangle inequality and the subadditivity of the superior,* $\sup_{\theta_i,\theta_j} |\sum_{j=1}^N J_{ij} f(\theta_i - \theta_j)| \leq \rho_i$*. Then, for any* $\epsilon > 0$*, choosing* $\frac{K_\mathrm{s}}{K} > \frac{\rho_i}{\epsilon}$ *results in*

$$|\sin(q\theta_i^\star)| = \left|\frac{K}{K_\mathrm{s}}\sum_{j=1}^{N} J_{ij} f(\theta_i^\star - \theta_j^\star)\right| < \epsilon,$$

*which implies that there exists* $k_i \in \mathbb{Z}^+$ *such that for any* $\epsilon \in (0, 1)$*,*

$$|q\theta_i^\star - k_i\pi| < \arcsin(\epsilon). \tag{13}$$

*If* $\frac{k_i+1}{2} \in \mathbb{Z}^+$ *for at least one* $i$*, say* $i = 1$*, then* $-1 < \cos(q\theta_1^\star) < \cos(k_i\pi + \arcsin(\epsilon)) = -\sqrt{1-\epsilon^2}$*. Thus,* $A_{11}(\theta^\star) = KD_{11}(\theta^\star) - qK_\mathrm{s}\cos(\theta_1^\star) > KD_{11}(\theta^\star) + qK_\mathrm{s}\sqrt{1-\epsilon^2}$*, which is positive if* $\frac{K_\mathrm{s}}{K} > -\frac{D_{11}(\theta_1^\star)}{q\sqrt{1-\epsilon^2}}$*. As a result, choosing* $\frac{K_\mathrm{s}}{K} > \max\left\{\frac{\rho_1}{\epsilon}, -\frac{D_{11}(\theta_1^\star)}{q\sqrt{1-\epsilon^2}}\right\}$ *makes* $\theta^\star$ *unstable. If* $\frac{k_i}{2} \in \mathbb{Z}^+$ *for all* $i$*, let* $\phi^\star = \mathrm{col}\left\{\frac{k_1\pi}{q}, \frac{k_2\pi}{q}, \ldots, \frac{k_N\pi}{q}\right\}$*. Note that* $\phi^\star$ *is a sampling point. Then,* (13) *holds for all* $i$ *by choosing* $\frac{K_\mathrm{s}}{K} > \max_i\{\frac{\rho_i}{\epsilon}\}$*, resulting in* $||\theta^\star - \phi^\star||_\infty = \max_i\{|\theta_i^\star - \phi_i^\star|\} < \frac{\arcsin(\epsilon)}{q}$*. Since* $\phi^\star$ *is asymptotically stable for* $\frac{K_\mathrm{s}}{K} > \frac{\lambda_N(D(\phi^\star))}{q}$*, there exists* $\epsilon_1 \in \left(0, \frac{\pi}{2q}\right)$ *such that* $\mathcal{D} = \{\theta \in \mathbb{T}^N : ||\theta - \phi^\star||_\infty < \epsilon_1\}$ *is an estimated attractive basin of* $\phi^\star$*. As a result,*

*choosing* $\frac{K_{\rm s}}{K} > \max\left\{\max_i \left\{\frac{\rho_i}{\epsilon}\right\}, \frac{\lambda_N(D(\phi^\star))}{q}\right\}$*, with* $\epsilon < \sin(q\epsilon_1)$*, makes* $\theta^\star$ *nonexistent, since such value of* $\frac{K_{\rm s}}{K}$ *will cause* $||\theta^\star - \phi^\star||_\infty < \epsilon_1$*, implying that* $\theta^\star$ *is located in the attractive basin of* $\phi^\star$*, which contradicts the definition of the attractive basin. This completes the proof.*

The attractive basin is an important dynamic property of asymptotically stable EPs. The next theorem characterizes the limit of the attractive basin for a sampling point as $\frac{K_{\rm s}}{K} \to \infty$.

**Theorem 4** *Consider the dynamics* (5)*. The attractive basin of each sampling point* $\theta^\star$ *converges to a hypercube* $\left(-\frac{\pi}{q}, +\frac{\pi}{q}\right)^N_{\theta^\star}$ *as* $\frac{K_{\rm s}}{K} \to \infty$*.*

**Proof 4** *By Theorem 3, all sampling points are asymptotically stable for large enough* $\frac{K_{\rm s}}{K}$*. Thus, the attractive basin of each sampling point exists for* $\frac{K_{\rm s}}{K} \to \infty$*. Consider the following dynamics*

$$\dot{\theta}_i = -K_{\rm s} \sin(q\theta_i), \tag{14}$$

*where* $\theta_i \in \mathbb{T}$*. It can be verified that* $(2q)^N$ *points belonging to* $\left\{\frac{k\pi}{q} : k = 0, 1, \ldots, 2q-1\right\}^N$ *constitute all EPs of* (14)*. In addition, a simple calculation shows that EPs belonging to* $\left\{\frac{2k\pi}{q} : k = 0, 1, \ldots, q-1\right\}^N$ *are asymptotically stable and others are unstable for any* $K_{\rm s} > 0$*. Thus, for each asymptotically stable EP* $\theta^\star$ *of* (14)*, the attractive basin is a hypercube* $\left(-\frac{\pi}{q}, +\frac{\pi}{q}\right)^N_{\theta^\star}$*. The potential function of* (14) *can be verified as*

$$W(\theta; K_{\rm s}) = -\frac{K_{\rm s}}{q}\left(\sum_{i=1}^N \cos(q\theta_i) + h\right),$$

*where* $h$ *is a constant. Recall that*

$$\begin{aligned} U(\theta; K_{\rm s}, K) &= -K\sum_{i<j} J_{ij}\left(2\sum_{m=1}^{q-1}(q-m)\cos(m(\theta_i - \theta_j))\right) - \frac{K_{\rm s}}{q}\left(\sum_{i=1}^N \cos(q\theta_i) + h\right) \\ &:= G(\theta; K) + W(\theta; K_{\rm s}) \end{aligned}$$

*is the potential function of* (5)*. In what follows, we analyze the potential function* $U(\theta)$ *for* $\frac{K_{\rm s}}{K} \to \infty$*. Without loss of generality, we fix* $K = 1$ *and let* $K_{\rm s} \to \infty$*. Specifically, we will show that* $\lim_{K_{\rm s}\to\infty} \frac{U(\theta; K_{\rm s}, 1)}{W(\theta; K_{\rm s})} = 1$ *uniformly with respect to* $\theta$*. Since* $\sum_{i=1}^N \cos(q\theta_i) \geq -N$*, we can choose* $h > N$ *such that* $W(\theta; K_{\rm s}) > 0$ *for all* $\theta$ *and* $K_{\rm s}$*, thus* $p := \inf_\theta \left(\sum_{i=1}^N \cos(q\theta_i) + h\right) > 0$*. Since* $G(\theta; 1)$ *is uniformly bounded with respect to* $\theta$*,* $\kappa := \sup_\theta |G(\theta; 1)| < \infty$*. For every* $\epsilon > 0$ *and* $\theta \in \mathbb{T}^N$*, choosing* $K_{\rm s} > \frac{q\kappa}{p\epsilon}$ *results in*

$$\sup_\theta \left|\frac{U(\theta; K_{\rm s}, 1)}{W(\theta; K_{\rm s})} - 1\right| = \sup_\theta \left|\frac{G(\theta; 1) + W(\theta; K_{\rm s})}{W(\theta; K_{\rm s})} - 1\right|$$

$$
\begin{aligned}
&= \sup_{\theta} \left| \frac{G(\theta;1)}{W(\theta;K_{\mathrm{s}})} \right| \\
&\le \sup_{\theta} \left| \frac{\kappa}{W(\theta;K_{\mathrm{s}})} \right| \\
&= \sup_{\theta} \left| \frac{\kappa}{\frac{K_{\mathrm{s}}}{q}\left(\sum_{i=1}^{N}\cos(q\theta_i)+h\right)} \right| \\
&< \sup_{\theta} \left| \frac{p\epsilon}{\left(\sum_{i=1}^{N}\cos(q\theta_i)+h\right)} \right| \\
&\le \epsilon
\end{aligned}
$$

*Thus,* $\lim_{K_{\mathrm{s}}\to\infty}\frac{U(\theta;K_{\mathrm{s}},1)}{W(\theta;K_{\mathrm{s}})}=1$ *uniformly with respect to* $\theta$*. This means that the potential landscapes of* (5) *and* (14) *converge to the same landscape as* $K_{\mathrm{s}}$ *increases. Note that the asymptotically stable EPs of* (14) *and the sampling points of* (5) *are the same. Finally, we conclude that the sampling point* $\theta^\star$ *of* (5) *has the attractive basin converging to a hypercube* $\left(-\frac{\pi}{q},+\frac{\pi}{q}\right)^N_{\theta^\star}$ *as* $\frac{K_{\mathrm{s}}}{K}\to\infty$*. This completes the proof.*

**Example.** We use numerical simulation to validate Theorem 4. Consider an OPM of three oscillators with $q=3$. Fig. 1 shows the phase portrait around $\theta^\star=\mathrm{col}\{0,0,0\}$ and $\phi^\star=\mathrm{col}\left\{0,\frac{2\pi}{3},0\right\}$ when $K=1, K_{\mathrm{s}}=50$. Fig. 2 shows the evolution of the phase portrait on the $(\theta_1,\theta_2)$ plane as $K_{\mathrm{s}}$ ranges from one to 50.

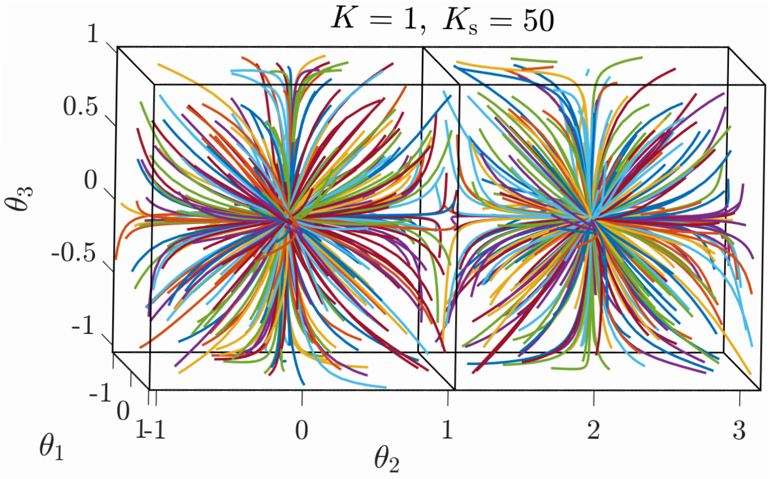


FIG. 1: Phase portrait

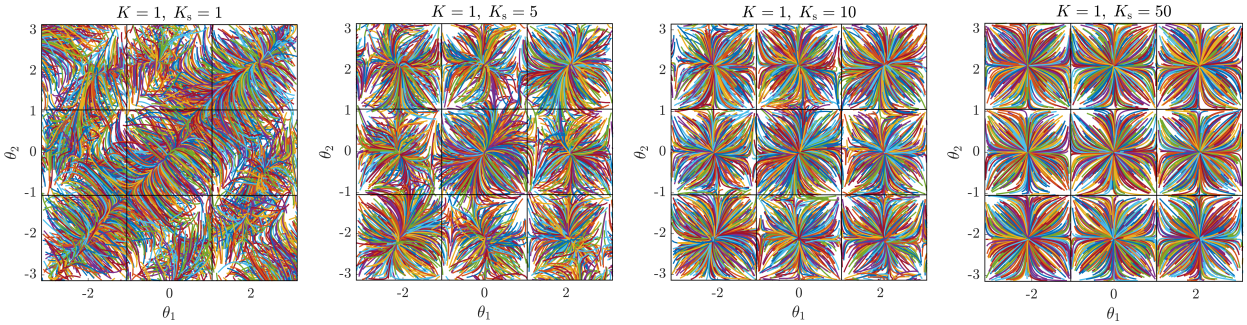


FIG. 2: Phase portraits of one dimension when $q = 3$. The attractive basins of EPs converge to a hypercube as $K_\mathrm{s}$ increases

## IV. QUANTIZATION OF A SAMPLE

By performing the dynamics (4), the distribution of $\theta_t$ coverages to a stationary distribution with the probability density function

$$\Pi(\theta) = Z^{-1}\mathrm{e}^{-\beta U(\theta)},$$

where $Z = \int_{\theta\in\mathbb{T}^N} \mathrm{e}^{-\beta U(\theta)}\mathrm{d}\theta$. Clearly, $\Pi(\theta)$ is continuous in $\theta$, which is different from the probability mass function $p(s)$ considered in the standard Potts model. For the Langevin model (4), sampling $\theta^\star$ is extremely ineffective, since the probability of the sampling point $\theta^\star$ is $\mathbb{P}(\theta^\star) = \int_{\theta=\theta^\star} \Pi(\theta)\mathrm{d}\theta = 0$. Therefore, we may take quantization on a sample $\theta_t$ to increase the probability of sampling points, which is also commonly used in Ising machines for combinatorial optimization problems. Here, the quantization we considered is that a sample $\theta_t$ falling within a hypercube $(-a,+a)^N_{\theta^\star}$ is assigned to the value of $\theta^\star$, where $a \in \left(0, \frac{\pi}{q}\right)$ is a constant, and $\theta^\star$ is a sampling point. After the quantization, the probability of the sampling point $\theta^\star$ occurring is

$$\begin{aligned}\mathbb{P}_\mathrm{q}(\theta^\star) &= \mathbb{P}(\theta_t : ||\theta_t - \theta^\star||_\infty < a) \\ &= Z^{-1}\int_{\theta_t\in(-a,+a)^N_{\theta^\star}} \mathrm{e}^{-\beta U(\theta_t)}\mathrm{d}\theta_t. \end{aligned} \tag{15}$$

When $a \to 0$, it can be shown that $\frac{\mathbb{P}_\mathrm{q}(\theta^\star)}{\mathbb{P}_\mathrm{q}(\phi^\star)} = \mathrm{e}^{\beta(U(\phi^\star)-U(\theta^\star))}$ (see Proposition 1 below), which is the Boltzmann ratio for the potential functions. As we discussed earlier, a smaller value of $a$ leads to a more ineffective discrete sampling. In contrast, a large value of $a$ improves the efficiency of discrete sampling, but cannot theoretically guarantee that the distribution (15) has the monotonicity property, that is, $U(\theta^\star) > U(\phi^\star)$ cannot theoretically guarantee that

$\mathbb{P}_{\mathrm{q}}(\theta^\star) < \mathbb{P}_{\mathrm{q}}(\phi^\star)$ for a large value of $a \in \left(0, \frac{\pi}{q}\right)$. In this section, we investigate whether a favorable trade-off exists between effective discrete sampling and the monotonicity property of the distribution (15). Our main result is shown in Theorem 5. Before we state the main result, we introduce a proposition for showing the property of (15) in an extreme case and a lemma for preliminary of the main result.

**Remark 3** *Let $\Theta$ be the set of $q^N$ sampling points. $\sum_{\theta^\star \in \Theta} \mathbb{P}_{\mathrm{q}}(\theta^\star) < 1$ since the region $\bigcup_{\theta^\star \in \Theta} (-a, +a)^N_{\theta^\star}$ is a subset of $\mathbb{T}^N$ for any $a \in \left(0, \frac{\pi}{q}\right)$. Therefore, in the finite set $\Theta$, we can define a renormalized discrete distribution over $\Theta$ as*

$$\tilde{\mathbb{P}}(\theta^\star) = \frac{\mathbb{P}_{\mathrm{q}}(\theta^\star)}{\sum_{\theta \in \Theta} \mathbb{P}_{\mathrm{q}}(\theta)}.$$

*This ensures that $\sum_{\theta \in \Theta} \tilde{P}(\theta) = 1$.*

**Proposition 1** *Consider two sampling points $\theta^\star$ and $\phi^\star$ of the OPM and the probability (15). Then,*

$$\lim_{a \to 0} \frac{\mathbb{P}_{\mathrm{q}}(\theta^\star)}{\mathbb{P}_{\mathrm{q}}(\phi^\star)} = \mathrm{e}^{\beta(U(\phi^\star) - U(\theta^\star))}.$$

**Proof 5** *Let $y = \theta - \theta^\star$. Then, we have $\Pi(y + \theta^\star) = \Pi(\theta)$. Since $\Pi(\theta)$ is differentiable, by the Taylor expansion with Lagrange remainder around $\theta^\star$,*

$$\Pi(y + \theta^\star) = \Pi(\theta^\star) + \nabla \Pi^{\mathrm{T}}(\theta^\star) y + R_2(y),$$

*where $|R_2(y)| \leq C||y||_2^2$ for small $||y||_2$ and a constant $C$. Then, for small enough $||y||_2$,*

$$\begin{aligned}
\int_{y \in (-a,+a)^N_{0_N}} \Pi(y + \theta^\star) \mathrm{d}y &= \int_{y \in (-a,+a)^N_{0_N}} \Pi(\theta^\star) \mathrm{d}y + \int_{y \in (-a,+a)^N_{0_N}} \nabla \Pi^{\mathrm{T}}(\theta^\star) y \mathrm{d}y \\
&\quad + \int_{y \in (-a,+a)^N_{0_N}} R_2(y) \mathrm{d}y \\
&= \int_{y \in (-a,+a)^N_{0_N}} \Pi(\theta^\star) \mathrm{d}y + \int_{y \in (-a,+a)^N_{0_N}} R_2(y) \mathrm{d}y \\
&= (2a)^N \Pi(\theta^\star) + O(a^{N+2}),
\end{aligned}$$

*where we have used the facts that $\nabla \Pi^{\mathrm{T}}(\theta^\star) y$ is an odd function with respect to $y$ and $(-a, +a)^N_{0_N}$ is a symmetric region with respect to $y$. In addition, we have also used the fact that, for small enough $||y||_2$,*

$$\left| \int_{y \in (-a,+a)^N_{0_N}} R_2(y) \mathrm{d}y \right| \leq \left| \int_{y \in (-a,+a)^N_{0_N}} C||y||_2^2 \mathrm{d}y \right|$$

$$
\begin{aligned}
&\leq \left| \int_{y \in (-a,+a)^N_{0_N}} CN||y||^2_\infty \mathrm{d}y \right| \\
&\leq \left| \int_{y \in (-a,+a)^N_{0_N}} CNa^2 \mathrm{d}y \right| \\
&= 2^N CNa^{N+2}.
\end{aligned}
$$

*Therefore,*

$$
\begin{aligned}
\lim_{a \to 0} \frac{\mathbb{P}_\mathrm{q}(\theta^\star)}{\mathbb{P}_\mathrm{q}(\phi^\star)} &= \lim_{a \to 0} \frac{\int_{y \in (-a,+a)^N_{0_N}} \Pi(y+\theta^\star)\mathrm{d}y}{\int_{y \in (-a,+a)^N_{0_N}} \Pi(y+\phi^\star)\mathrm{d}y} \\
&= \lim_{a \to 0} \frac{(2a)^N \Pi(\theta^\star) + O(a^{N+2})}{(2a)^N \Pi(\phi^\star) + O(a^{N+2})} \\
&= \lim_{a \to 0} \frac{\Pi(\theta^\star) + \frac{O(a^{N+2})}{(2a)^N}}{\Pi(\phi^\star) + \frac{O(a^{N+2})}{(2a)^N}} \\
&= \frac{\Pi(\theta^\star)}{\Pi(\phi^\star)} \\
&= \mathrm{e}^{\beta(U(\phi^\star) - U(\theta^\star))}.
\end{aligned}
$$

*This completes the proof.*

**Lemma 1** *Consider a sampling point $\theta^\star$ and a hypercube $(-a,+a)^N_{\theta^\star}$. For any $a \in \left(0, \frac{\pi}{2q}\right)$, the potential function (2) is strongly convex in $(-a,+a)^N_{\theta^\star}$ for large enough $\frac{K_\mathrm{s}}{K}$. In addition, $\theta^\star$ is the unique minimum of $U(\theta)$ in $(-a,+a)^N_{\theta^\star}$.*

**Proof 6** *The Hessian matrix of $U(\theta)$ is given by*

$$
\nabla^2 U(\theta) = -A(\theta) = -KD(\theta) + qK_\mathrm{s}\Delta(\theta),
$$

*where $D(\theta)$ is a symmetric matrix given in Proof of Theorem 3, and $\Delta(\theta)$ is a diagonal matrix whose diagonal is $\Delta_{ii}(\theta) = \cos(q\theta_i)$. Since $\theta^\star_i \in \left\{\frac{2k\pi}{q} : k = 0, 1, \ldots, q-1\right\}$ and $a \in \left(0, \frac{\pi}{2q}\right)$, it can be verified that $\cos(q\theta_i) > 0$ for any $\theta_i \in [\theta^\star_i - a, \theta^\star_i + a]$. Given a point $\theta \in [-a,+a]^N_{\theta^\star}$, let $\kappa = \max_i\{|D_{ii}(\theta)|\}$, $\varsigma = \max_i\{\sum_{j \neq i, j=1}^N |D_{ij}(\theta)|\}$, and $g = \min_i\{\Delta_{ii}(\theta)\}$. Note that $g > 0$. Choosing $\frac{K_\mathrm{s}}{K} > \frac{\kappa+\varsigma}{qg}$ ensures that $\nabla^2 U(\theta)$ is a diagonal dominance matrix for any $\theta \in [-a,+a]^N_{\theta^\star}$, where $a \in (0, \frac{\pi}{2q})$. Note that $\nabla^2 U(\theta)$ is symmetric. By Gershgorin Disc Theorem, we see that $\nabla^2 U(\theta)$ is positive definite, and therefore $U(\theta)$ is strictly convex in $[-a,+a]^N_{\theta^\star}$ as $[-a,+a]^N_{\theta^\star}$ is the convex set. Given that the hypercube $[-a,+a]^N_{\theta^\star}$ is a compact set, $U(\theta)$ is strongly convex in $[-a,+a]^N_{\theta^\star}$. Since $(-a,+a)^N_{\theta^\star} \subset [-a,+a]^N_{\theta^\star}$, $U(\theta)$ is strongly*

*convex in* $(-a,+a)^N_{\theta^\star}$. *By Theorem 2,* $\nabla U(\theta^\star) = 0_N$*, and therefore* $\theta^\star$ *is the unique minimum of* $U(\theta)$ *in* $(-a,+a)^N_{\theta^\star}$. *This completes the proof.*

**Theorem 5** *Consider the potential function* (2) *and the distribution* (15) *at the sampling points. Let* $\theta^\star$ *and* $\phi^\star$ *be two sampling points. Let* $U(\theta^\star) > U(\phi^\star)$ *and* $d = U(\theta^\star) - U(\phi^\star)$. *There exists a constant* $\mu > 0$ *and* $\delta = \min\left\{\sqrt{\frac{2d}{\mu}}, \frac{\pi}{2q}\right\}$ *such that for all* $a \in (0,\delta)$ *and large enough* $\frac{K_s}{K}$, $\mathbb{P}_q(\theta^\star) < \mathbb{P}_q(\phi^\star)$.

**Proof 7** *Let* $\gamma^\star = \theta^\star - \phi^\star$. *Then* $U(\theta)$ *in* $(-a,+a)^N_{\phi^\star}$ *is pointwise equal to* $U(\theta - \gamma^\star)$ *in* $(-a,+a)^N_{\theta^\star}$. *Let* $W(\theta) = U(\theta - \gamma^\star)$. *By Lemma 1, we can choose* $\frac{K_s}{K}$ *large enough such that both* $U(\theta)$ *and* $W(\theta)$ *are strongly convex in* $(-a,+a)^N_{\theta^\star}$ *for any* $a \in \left(0, \frac{\pi}{2q}\right)$*, where* $\theta^\star$ *is the common unique minimum. Let* $F(\theta) = U(\theta) - W(\theta)$ *and* $d = F(\theta^\star)$. *Note that* $W(\theta^\star) = U(\phi^\star) < U(\theta^\star)$*, and hence* $d > 0$. *Since* $U(\theta)$ *is strongly convex for* $\theta \in (-a,+a)^N_{\theta^\star}$ *with* $a \in \left(0, \frac{\pi}{2q}\right)$*, there exists* $m_1 > 0$ *such that for any* $\theta \in (-a,+a)^N_{\theta^\star}$ *with* $a \in \left(0, \frac{\pi}{2q}\right)$,

$$\begin{aligned} U(\theta) &\geq U(\theta^\star) + \nabla U(\theta^\star)^{\mathrm{T}}(\theta - \theta^\star) + \frac{m_1}{2}||\theta - \theta^\star||_2^2 \\ &\geq U(\theta^\star) + \frac{m_1}{2}||\theta - \theta^\star||_\infty^2. \end{aligned} \tag{16}$$

*By the Taylor expansion with the Lagrange form of reminder,* $W(\theta)$ *can be expressed as*

$$\begin{aligned} W(\theta) &= W(\theta^\star) + \nabla W(\theta^\star)^{\mathrm{T}}(\theta - \theta^\star) + \frac{1}{2}(\theta - \theta^\star)^{\mathrm{T}}\nabla^2 W(\xi)(\theta - \theta^\star) \\ &= W(\theta^\star) + \frac{1}{2}(\theta - \theta^\star)^{\mathrm{T}}\nabla^2 W(\xi)(\theta - \theta^\star), \end{aligned} \tag{17}$$

*for some* $\xi$ *lies on the interval between* $\theta$ *and* $\theta^\star$. *Let* $m_2 = \max_{\theta \in [-a,+a]^N_{\theta^\star}} \lambda_N(\nabla^2 W(\theta))$. *In view of* (16) *and* (17)*, we have*

$$\begin{aligned} F(\theta) &= U(\theta) - W(\theta) \\ &\geq U(\theta^\star) - W(\theta^\star) + \frac{m_1}{2}||\theta - \theta^\star||_\infty^2 - \frac{m_2}{2}||\theta - \theta^\star||_2^2 \\ &= d + \frac{m_1}{2}||\theta - \theta^\star||_\infty^2 - \frac{m_2}{2}||\theta - \theta^\star||_2^2 \\ &\geq d + \frac{m_1 - m_2 N}{2}||\theta - \theta^\star||_\infty^2, \end{aligned}$$

*where we have used the fact that* $||\theta - \theta^\star||_2^2 \leq N||\theta - \theta^\star||_\infty^2$. *If* $m_1 \geq m_2 N$*, we have* $F(\theta) > 0$ *for all* $\theta \in (-a,+a)^N_{\theta^\star}$ *with* $a \in \left(0, \frac{\pi}{2q}\right)$. *If* $m_1 < m_2 N$, $F(\theta) > 0$ *for*

$$\theta \in \left\{\theta : ||\theta - \theta^\star||_\infty < \sqrt{\frac{2d}{m_2 N - m_1}} := \sqrt{\frac{2d}{\mu}}\right\}.$$

*In other words, there exist* $\mu > 0$ *and* $\delta = \min\left\{\sqrt{\frac{2d}{\mu}}, \frac{\pi}{2q}\right\}$ *such that for any* $a \in (0, \delta)$ *and any* $\theta \in (-a, +a)^N_{\theta^\star}$*,* $F(\theta) > 0$*, that is,* $U(\theta) > W(\theta) = U(\theta - \gamma^\star)$*. Thus,* $\mathrm{e}^{-\beta U(\theta)} < \mathrm{e}^{-\beta U(\theta-\gamma^\star)}$ *for any* $\theta \in (-a, +a)^N_{\theta^\star}$*. Then, by the monotonicity of the integral,*

$$\begin{aligned}
\frac{\mathbb{P}_{\mathrm{q}}(\theta^\star)}{\mathbb{P}_{\mathrm{q}}(\phi^\star)} &= \frac{\mathbb{P}_{\mathrm{q}}(\theta^\star)}{\mathbb{P}_{\mathrm{q}}(\theta^\star - \gamma^\star)} \\
&= \frac{\int_{\theta \in (-a,+a)^N_{\theta^\star}} Z^{-1} \mathrm{e}^{-\beta U(\theta)} \mathrm{d}\theta}{\int_{\theta \in (-a,+a)^N_{\theta^\star - \gamma^\star}} Z^{-1} \mathrm{e}^{-\beta U(\theta)} \mathrm{d}\theta} \\
&= \frac{\int_{\theta \in (-a,+a)^N_{\theta^\star}} \mathrm{e}^{-\beta U(\theta)} \mathrm{d}\theta}{\int_{\theta \in (-a,+a)^N_{\theta^\star - \gamma^\star}} \mathrm{e}^{-\beta U(\theta)} \mathrm{d}\theta} \\
&= \frac{\int_{\theta \in (-a,+a)^N_{\theta^\star}} \mathrm{e}^{-\beta U(\theta)} \mathrm{d}\theta}{\int_{\theta \in (-a,+a)^N_{\theta^\star}} \mathrm{e}^{-\beta U(\theta - \gamma^\star)} \mathrm{d}\theta} \\
&< 1.
\end{aligned}$$

*This completes the proof.*

To demonstrate Theorem 5, consider an OPM of two oscillators with $q = 3$. The coupling weight $J_{12} = -1$. Fix $K = 1$ and $K_{\mathrm{s}} = 15$. Consider $\theta^\star = \{0, 0\}$ and $\phi^\star = \{\frac{2\pi}{3}, 0\}$. A simple calculation shows that $U(\theta^\star) = -8$ and $U(\phi^\star) = -11$. Let $\gamma^\star = \theta^\star - \phi^\star$ and $W(\theta) = U(\theta - \gamma^\star)$. We have $W(\theta)$ in the region of $\left(-\frac{\pi}{3}, +\frac{\pi}{3}\right)^2_{\theta^\star}$ pointwise equal to $U(\theta)$ in the region of $\left(-\frac{\pi}{3}, +\frac{\pi}{3}\right)^2_{\phi^\star}$. Clearly, $W(\theta^\star) = U(\phi^\star) = -11$. Fig. 3 shows the manifolds of $U(\theta)$ and $W(\theta)$ in the region of $\left(-\frac{\pi}{3}, +\frac{\pi}{3}\right)^2_{\theta^\star}$. We observe that $U(\theta) > W(\theta)$ in the black rectangle, where the black rectangle is $\left(-\frac{\pi}{6}, +\frac{\pi}{6}\right)^2_{\theta^\star}$.

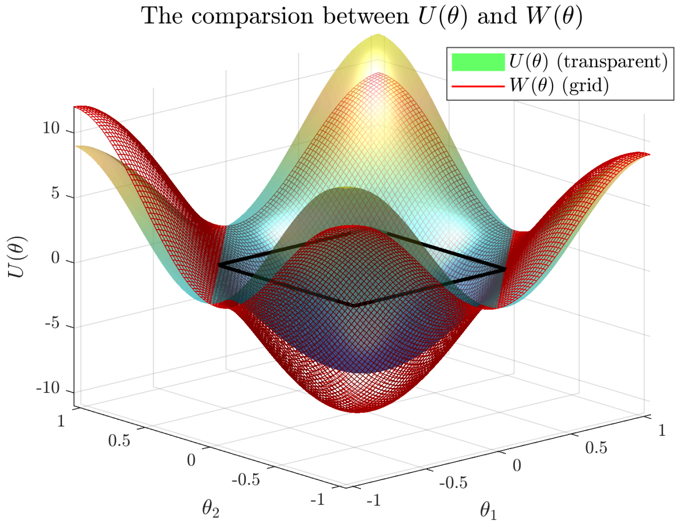


FIG. 3: The manifolds of $U(\theta)$ and $W(\theta)$ in the region of $\left(-\frac{\pi}{3},+\frac{\pi}{3}\right)^2_{\theta^\star}$; $U(\theta) > W(\theta)$ in the region of $\left(-\frac{\pi}{6},+\frac{\pi}{6}\right)^2_{\theta^\star}$ (black rectangle).
